# Supplementary material for: LSH methods for data deduplication in a Wikipedia artificial dataset
Source: arXiv:2112.11478 source file (2021-12-10)
Supplement: Supplementary file 1 [file 06_appendix.tex]

\section{Appendix}

\subsection{Word Error Rate Analysis}\label{sec:wer-full}

In Table~\ref{tab:full-wer} we provide the full table of word error rates from Section~\ref{subsec:anomaly-detection}.

% \begin{wraptable}{r}{0.28\textwidth}
% \centering
% \begin{adjustbox}{width=0.28\textwidth}
% \begin{tabular}{lrrr}
% \toprule
%         Word &  \# Clips & Near & Far \\
% \midrule
%          may &     7551 &       4\% &     32\% \\
%          did &    14353 &      32\% &     32\% \\
%         soon &     3269 &       6\% &     34\% \\
%       shirt &     1299 &       0\% &     54\% \\
%       style &     1760 &       0\% &     12\% \\
%       taken &     1734 &       0\% &     12\% \\
%       stood &     1739 &       0\% &     22\% \\
%       watch &     1476 &       4\% &     28\% \\
%       happy &     2095 &       2\% &      8\% \\
%       entire &     1354 &       0\% &     12\% \\
%       engine &     1043 &       0\% &     18\% \\
%       nature &     1018 &       0\% &     12\% \\
%       you've &     1886 &       0\% &     26\% \\
%      reading &     1594 &       8\% &     58\% \\
%      village &     2801 &       0\% &     34\% \\
%      outside &     2075 &       0\% &      2\% \\
%      strange &     1720 &       0\% &     18\% \\
%      current &     1836 &      10\% &      4\% \\
%      musical &     1108 &       0\% &     16\% \\
%     followed &     1307 &       0\% &     10\% \\
%     learning &     1075 &       2\% &     18\% \\
%     provided &     1627 &       0\% &      4\% \\
%   difficult &     1771 &       0\% &      8\% \\
%   political &     1474 &       0\% &      8\% \\
%  performance &     1007 &       6\% &     12\% \\
% \bottomrule
% \end{tabular}
% \end{adjustbox}
% \caption{Word error rates (WER) by outlier metric.} 
% \end{wraptable}
\begin{table}
\centering
\caption{Word error rates (WER) by outlier metric.} 
\begin{tabular}{lrrr}
\toprule
        Word &  \# Clips & Near WER & Far WER \\
\midrule
         may &     7551 &       4\% &     32\% \\
         did &    14353 &      32\% &     32\% \\
        soon &     3269 &       6\% &     34\% \\
       shirt &     1299 &       0\% &     54\% \\
       style &     1760 &       0\% &     12\% \\
       taken &     1734 &       0\% &     12\% \\
       stood &     1739 &       0\% &     22\% \\
       watch &     1476 &       4\% &     28\% \\
      happy &     2095 &       2\% &      8\% \\
      entire &     1354 &       0\% &     12\% \\
      engine &     1043 &       0\% &     18\% \\
      nature &     1018 &       0\% &     12\% \\
      you've &     1886 &       0\% &     26\% \\
     reading &     1594 &       8\% &     58\% \\
     village &     2801 &       0\% &     34\% \\
     outside &     2075 &       0\% &      2\% \\
     strange &     1720 &       0\% &     18\% \\
     current &     1836 &      10\% &      4\% \\
     musical &     1108 &       0\% &     16\% \\
    followed &     1307 &       0\% &     10\% \\
    learning &     1075 &       2\% &     18\% \\
    provided &     1627 &       0\% &      4\% \\
   difficult &     1771 &       0\% &      8\% \\
   political &     1474 &       0\% &      8\% \\
 performance &     1007 &       6\% &     12\% \\
\bottomrule
\end{tabular}
\label{tab:full-wer}
\end{table}

\subsection{Semantic classification on keywords}\label{sec:full-semantic}

We provide additional data on semantic classification in English, Spanish, and Arabic in Table~\ref{sec:full-semantic}, in reference to our discussion in Sec.~\ref{sec:keyword-characterization}

\begin{table}[t!]
	\centering
	\centering
	\caption{Semantic keyword characterization in English, Spanish and Arabic via zero-shot multilingual NLI with representative samples. Number of clips (\#C) and keywords (\#K). Sorted by \#K in English.}
	\resizebox{\textwidth}{!}{
		\begin{tabular}{|c||c|c|c||c|c|c||c|c|c|} 
			\hline
			Category & \# C & \# K & English & \#C & \#K & Spanish & \#C & \#K & Arabic \\ \hline  \hline 
			Event   &%
			3M &    1K &        \multicolumn{1}{c||}{\begin{tabular}[c]{@{}c@{}}School, Preakness, \\Commanded\end{tabular}}  &%
			153K &   238 &             \multicolumn{1}{c||}{\begin{tabular}[c]{@{}c@{}}Campeonato, Episodio,\\Eurovisión\end{tabular}} &%
			2K &    30 &            \begin{otherlanguage*}{arabic}ي قال, حصل, يحبها \end{otherlanguage*} \\  \hline
			\multicolumn{1}{|c||}{\begin{tabular}[c]{@{}c@{}} Human\\activity \end{tabular}} &%
			1M &   820 & \multicolumn{1}{c||}{\begin{tabular}[c]{@{}c@{}} Shooting, Prefers,\\Attacking\end{tabular}} &%
			78K &   211 &      \multicolumn{1}{c||}{\begin{tabular}[c]{@{}c@{}}    Expandiendo, Visitando,\\Carpintería\end{tabular}} &%
			1K &    28 &    \begin{otherlanguage*}{arabic}ستغادر, المشتري, لنغني \end{otherlanguage*}  \\ \hline 
			Location &%
			391K &   379 &             \multicolumn{1}{c||}{\begin{tabular}[c]{@{}c@{}} Home, County, \\Desert\end{tabular}}  &
			213K &   324 &               \multicolumn{1}{c||}{\begin{tabular}[c]{@{}c@{}} Zona, Pueblo, \\Marítima\end{tabular}}  &
			333 &    14 &  \begin{otherlanguage*}{arabic}ي قال, حصل, يحبها \end{otherlanguage*}  \\  \hline
			Name &%
			327K &   303 &                \multicolumn{1}{c||}{\begin{tabular}[c]{@{}c@{}} Margot, Cooney, \\Alvin\end{tabular}}  &
			30K &   128 &               \multicolumn{1}{c||}{\begin{tabular}[c]{@{}c@{}} Eduardo, Peter, \\Francisco\end{tabular}}  &
			1K &    24 &          \begin{otherlanguage*}{arabic}انا, ساءبقى, اءدري \end{otherlanguage*}  \\  \hline
			Animal &%
			131K &   281 &                  \multicolumn{1}{c||}{\begin{tabular}[c]{@{}c@{}} Sheep, Camel, \\Muzzle\end{tabular}}  &
			99K &   137 &                  \multicolumn{1}{c||}{\begin{tabular}[c]{@{}c@{}} Águila, Especies, \\Jaguar\end{tabular}}  &
			1K &    25 &          \begin{otherlanguage*}{arabic}فيه, تفاحة, باللون \end{otherlanguage*}  \\  \hline
			Number &     301K &   279 &           \multicolumn{1}{c||}{\begin{tabular}[c]{@{}c@{}} Second, Six, \\Stringent, \end{tabular}}  &
			31K &    75 &        \multicolumn{1}{c||}{\begin{tabular}[c]{@{}c@{}} Multiplicar, Primero, \\Estadísticos\end{tabular}}  &
			493 &    17 &           \begin{otherlanguage*}{arabic}عشرة, واحد, ثلاثة \end{otherlanguage*}  \\ \hline
			\multicolumn{1}{|c||}{\begin{tabular}[c]{@{}c@{}} General\\reference\end{tabular}}  &%
			113K &   220 &         \multicolumn{1}{c||}{\begin{tabular}[c]{@{}c@{}} Understand, Generally, \\Trivial\end{tabular}}  &
			216K &   319 &  \multicolumn{1}{c||}{\begin{tabular}[c]{@{}c@{}} Recomendaciones,\\ Recompensa, Frecuencias\end{tabular}}  &
			185 &     8 &       \begin{otherlanguage*}{arabic}طريقة, القانون, التعب \end{otherlanguage*}  \\ \hline
			\multicolumn{1}{|c||}{\begin{tabular}[c]{@{}c@{}} Common\\words\end{tabular}}  &%
			218K &   217 &                  \multicolumn{1}{c||}{\begin{tabular}[c]{@{}c@{}} Often, Popular, \\Usually\end{tabular}}  &
			56K &   172 &              \multicolumn{1}{c||}{\begin{tabular}[c]{@{}c@{}} Tambien, Ademas, \\ Biográfico\end{tabular}}  &
			206 &     7 &           \begin{otherlanguage*}{arabic}عديدة, تمطر, مخطئ  \end{otherlanguage*} \\ \hline
			City &%
			106K &   212 &    \multicolumn{1}{c||}{\begin{tabular}[c]{@{}c@{}} York, London, \\California\end{tabular}}  &
			34K &    94 &                  \multicolumn{1}{c||}{\begin{tabular}[c]{@{}c@{}} Madrid, Berlín, \\Oxford\end{tabular}}  &
			49 &     4 &    \begin{otherlanguage*}{arabic}اءيطاليا, بيكاسو, البلدة  \end{otherlanguage*} \\ \hline
			Technology &%
			52K &   191 &     \multicolumn{1}{c||}{\begin{tabular}[c]{@{}c@{}} Gramophone, \\Television, Videotape\end{tabular}}  &
			21K &   106 &                  \multicolumn{1}{c||}{\begin{tabular}[c]{@{}c@{}} Automotriz, Lego, \\Sensor\end{tabular}}  & 
			92 &     5 &  \begin{otherlanguage*}{arabic} التلفاز, السيارات, الاءخير  \end{otherlanguage*}  \\ \hline
			Culture &%
			52K &   180 &          \multicolumn{1}{c||}{\begin{tabular}[c]{@{}c@{}} Popularize, Music, \\Style\end{tabular}}  &
			15K &    86 &        \multicolumn{1}{c||}{\begin{tabular}[c]{@{}c@{}} Tradicional, Concertista, \\Cantante\end{tabular}}  &
			57 &     4 &        \begin{otherlanguage*}{arabic}الصينية, بمهارة, فوق  \end{otherlanguage*}  \\ \hline
			Language &%
			92K &   132 &           \multicolumn{1}{c||}{\begin{tabular}[c]{@{}c@{}} Arabic, English, \\Words\end{tabular}}  &
			8K &    69 &                   \multicolumn{1}{c||}{\begin{tabular}[c]{@{}c@{}} Español, Lengua, \\Inglesa\end{tabular}}  &
			98 &     7 & \begin{otherlanguage*}{arabic}اللغة, بالاءنجليزية, ياباني  \end{otherlanguage*}  \\ \hline
			Game &%
			48K &   131 &            \multicolumn{1}{c||}{\begin{tabular}[c]{@{}c@{}} Play, Kirby's, \\Football\end{tabular}}  &
			8K &    46 &                  \multicolumn{1}{c||}{\begin{tabular}[c]{@{}c@{}} Deportes, Partido, \\Equipo\end{tabular}}  &
			- & - & - \\ \hline
			Political &%
			37K &   124 &      \multicolumn{1}{c||}{\begin{tabular}[c]{@{}c@{}} Impeached, Campaigns, \\Democrats\end{tabular}}  &
			13K &    86 &   \multicolumn{1}{c||}{\begin{tabular}[c]{@{}c@{}} Intendentes, Libertario, \\Poder\end{tabular}}  &
			2K &    32 &          \begin{otherlanguage*}{arabic}رؤية, المفضل, معي  \end{otherlanguage*}   \\ \hline
			History &%
			52K &   119 &  \multicolumn{1}{c||}{\begin{tabular}[c]{@{}c@{}} Stories, Ancient, \\Roman\end{tabular}}  &
			12K &    73 &         \multicolumn{1}{c||}{\begin{tabular}[c]{@{}c@{}} Conquistas,\\Emperador, Históricas\end{tabular}}  &
			257 &     8 &          \begin{otherlanguage*}{arabic} قبل, اءتذكر, عمرها   \end{otherlanguage*}\\ \hline
		\end{tabular}
	}
	\label{tab:zero-shot-full}
\end{table}
